# Supplementary material for: Efficient Long-Range Machine Learning Force Fields for Liquid and Materials Properties
Source: arXiv:2505.06462 ancillary file (2025-08-01)
Supplement: Supplementary file 1 [file supporting_information.pdf]

# Supplementary Information: Efficient Long-Range Machine Learning Force Fields for Liquid and Materials Properties

John L. Weber,[†] Rishabh D. Guha,[†] Garvit Agarwal,[†] Yujing Wei,[†,‡] Aidan A. Fike,[†] Xiaowei Xie,[¶] James Stevenson,[†] Biswajit Santra,[†] Richard A. Friesner,[‡] Karl Leswing,[†] Mathew D. Halls,[§] Robert Abel,[†] and Leif D. Jacobson[*,¶]

†*Schrödinger Inc., 1540 Broadway, 24th floor, New York, NY 10036*

‡*Department of Chemistry, Columbia University, 3000 Broadway, New York, NY 10027*

¶*Schrödinger Inc., 101 SW Main Street, Suite 1300, Portland, OR 97204*

§*Schrödinger Inc., 9868 Scranton Road, Suite 3200 San Diego, CA 92121*

E-mail: leif.jacobson@schrodinger.com

# Contents


**S1 Monoelemental Crystal Test** **S3**

**S2 TorsionTest2000 details** **S5**

**S3 Relative tautomer test details** **S5**

**S4 X23b cohesive energies** **S6**

**S5 Organic crystal test details** **S6**

**S6 Liquid Solvent Densities** **S6**

**S7 TorsionNet500 DLPNO-CCSD(T) details** **S11**

**S8 Water hydration free energy details** **S11**

**S9 NaCl electric response** **S12**

**S10 Phonon Calculations** **S12**

**S11 LiAlO2 data** **S13**

**References** **S13**

# S1 Monoelemental Crystal Test

**Table S1: List of elements and their associated MP-IDs**

| Element | MP-IDs |
|---|---|
| Ac | mp-1183057 |
| Ag | mp-2646971 |
| Al | mp-1244953, mp-1245067, mp-1245129, mp-1245152, mp-1245307, mp-2647008 |
| As | mp-1096826, mp-1182332, mp-1238842 |
| Au | mp-1238808, mp-2647062 |
| Ba | mp-1096835, mp-1096840, mp-1977763 |
| Be | mp-1008501 |
| Bi | mp-1067758, mp-1078637, mp-1182070, mp-1182248, mp-23157, mp-567379, mp-568087, mp-568714, mp-569358 |
| B | mp-1104251, mp-1182425, mp-1196985, mp-729184 |
| Br | mp-1120813, mp-23154 |
| Ca | mp-1078638, mp-1227541, mp-166 |
| Cd | mp-2647135 |
| C | mp-1040425, mp-1097832, mp-1147718, mp-1182684, mp-1196583, mp-1197903, mp-1244913, mp-2516584, mp-2646980, mp-2647017, mp-568363, mp-624889, mp-632329, mp-683919, mp-723638, mp-731594 |
| Cr | mp-1192789 |
| Cs | mp-1007976, mp-1096915, mp-573579 |
| F | mp-1067793, mp-760482 |
| Ge | mp-1061054, mp-1067619, mp-1224349, mp-128, mp-148 |
| Hg | mp-1077098, mp-1096992, mp-1181096, mp-1224431, mp-2629196, mp-569289, mp-982872 |
| H | mp-632172, mp-754417 |
| I | mp-23153, mp-601148 |
| Ir | mp-2647032 |
| K | mp-1068966, mp-1078640, mp-1080043, mp-1199937, mp-573691 |
| Li | mp-1103107 |
| Mn | mp-2647025 |
| Mo | mp-1066523, mp-1180307, mp-1181019, mp-1190217, mp-2647013 |
| Na | mp-1079952, mp-1221597, mp-974920, mp-999501 |

| | |
|---|---|
| Nb | mp-1094120, mp-1104341, mp-2647103 |
| N | mp-1061298, mp-754514 |
| O | mp-1056831, mp-1058623, mp-1065697, mp-1102442, mp-1180008, mp-1180036, mp-12957, mp-2421172, mp-607540, mp-734188 |
| Os | mp-2647031 |
| Pb | mp-1102666 |
| Pd | mp-2646977 |
| P | mp-1120743 |
| Pr | mp-567630 |
| Pt | mp-2646979, mp-2647022 |
| Pu | mp-1055423, mp-1179962 |
| Rb | mp-1063817, mp-1179656, mp-1179802, mp-639736, mp-640416, mp-656615 |
| Re | mp-2647037 |
| Rh | mp-1239193, mp-2646993 |
| Sb | mp-1104795, mp-1179605, mp-1179613, mp-1179618, mp-1236935, mp-567409, mp-632286 |
| Sc | mp-1055932, mp-1056366, mp-1064244, mp-1977495 |
| Si | mp-1001113, mp-1079649, mp-1201492, mp-1244933, mp-1244971, mp-1244990, mp-1245041, mp-1245242, mp-1403870, mp-168, mp-2351841, mp-644693, mp-676011, mp-988210 |
| S | mp-1065250, mp-1179639, mp-1179641, mp-1179643, mp-1196831, mp-655141, mp-666931 |
| Sn | mp-1056308, mp-1179414, mp-623511 |
| Sr | mp-1179325 |
| Ta | mp-2647044, mp-697196 |
| Te | mp-1178952 |
| Ti | mp-1244924, mp-1245006, mp-1245164, mp-1245170, mp-1245320 |
| U | mp-1077335, mp-1197206, mp-1200324, mp-1981700, mp-1983234 |
| V | mp-2647074 |
| W | mp-1065340, mp-1191581, mp-1216274, mp-2646990 |
| Xe | mp-972256 |
| Zn | mp-1244987, mp-1245093, mp-1245184, mp-1245266, mp-2646972, mp-2647117 |
| Zr | mp-1178608 |

# S2 TorsionTest2000 details

To cover ionic systems and a wider list of elements. We downloaded traunches of ZINC20[1] up to 300 Dalton. Out of this set we selected 500 molecules randomly, including 100 ionic molecules and 100 molecules with at least one of the elements Br, Si, B or P. These molecules were then fragmented to retain the character of a central torsion and deduplicated. For each fragment, we perform a conformational search with MacroModel and rank the conformers with a preliminary Organic_MPNICE model. The lowest energy conformer is selected and a relaxed torsion scan is performed with the $\omega$B97X-D3BJ/def2-TZVPD functional, with 24 points per torsion scan using the Jaguar electronic structure program in the pseudo-spectral approximation. For consistency with training data we perform single point energy evaluation with Psi4 using the RI approximation. After filtering reacted geometries and unconverged optimizations we are left with 2109 torsion scans covering the elements H B C N O S F P Cl Br Si, giving a diverse and challenging torsion set. For each torsion scan we compute the RMSD in relative energies, where the zero of energy is again defined by the lowest energy DFT structure.

# S3 Relative tautomer test details

Previously we had reported on the ability of QRNN models to reproduce the gas phase relative tautomer energies relative to our previous level of theory, $\omega$B97X-D/6-31G(d).[2] We had optimized tautomer pairs from the publicly available tautobase dataset[3] corresponding to elements supported by QRNN. Here, we refine this test by re-optimizing these pairs at the $\omega$B97X-D3BJ/def2-TZVPD level utilizing Jaguar in the pseudo-spectral approximation. For consistency with training data we perform single point energy evaluation with Psi4 using the RI approximation. Out of 1546 tautomer pairs compatible with QRNN we were unable to tightly converge the optimization in 47 cases, resulting in 1499 pairs.

# S4 X23b cohesive energies

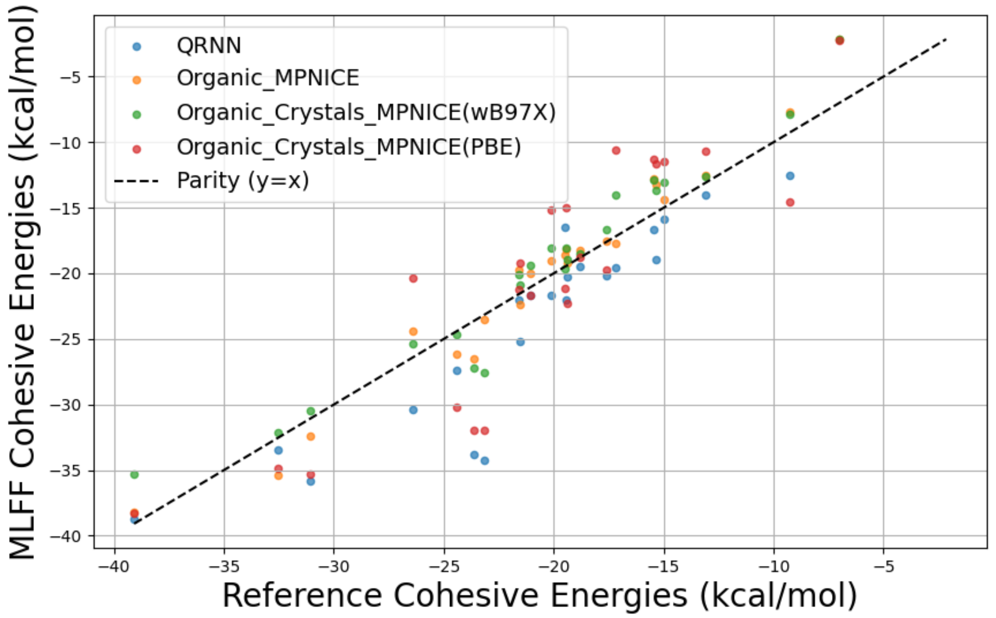


Figure S1: X23b lattice energy correlation for MPNICE models and QRNN. Note that QRNN excludes one case which obtained a cohesive energy of <-4000 kcal/mol.

# S5 Organic crystal test details

Recently, some of us have reported on a CSP protocol and tested it on 65 organic molecules of varying complexity.[4] In the course of that work we performed many PBE-D3 optimizations of organic crystal structures and we use a subset of 20 systems which were particularly challenging for our prior QRNN model. When performing DFT ranking of crystal structures we perform loose optimization (max force component is less than 0.26 eV/Å) of structures with PBE-D3, of a short list of structures from our MLFF, at the time, QRNN.[4] Here we use this list of structures to evaluate the error in relative energy, normalized to the number of molecules. The number of structures in each set varies between 196 (QQQAUG) and 3011 (BEDMIG) and as in our prior work, we restrict our attention to Z'=1 polymorphs.

# S6 Liquid Solvent Densities

We construct periodic simulation cells containing as close to 1000 atoms as possible, given the size of the molecule. These cells are optimized then equilibrated in the NVT ensemble for 100 ps and further equilibrated for 100 ps in the NPT ensemble prior to a 1 ns NPT simulation at the experimental temperature in order to determine the average mass density of each system. The production MD simulations were performed with the Desmond MD engine.

**Table S2: Liquid solvent densities for organic models. Italics indicate the system vaporized over the course of the simulation.**

| System | T (K) | Expt | QRNN | Organic_MPNICE | Organic_Crystals_MPNICE(wB97X) | Organic_Crystals_MPNICE(PBE) |
|---|---|---|---|---|---|---|
| 1-butanol | 298 | 0.8095 | 0.9155 | 0.7804 | 0.7361 | 0.6285 |
| 1-propanol | 303 | 0.7997 | 0.9087 | 0.7533 | 0.7275 | 0.6327 |
| 1,2-dichloroethane | 303 | 1.2454 | 1.6044 | 1.2184 | 1.1501 | 0.7074 |
| 1,2-dimethoxy-ethane | 303 | 0.8637 | 1.0237 | 0.8222 | 0.7417 | 0.5617 |
| 1,2-dimethylbenzene(o-xylene) | 278 | 0.8802 | 0.9738 | 0.880783 | 0.8022 | 0.6892 |
| 1,4-dioxane | 298 | 1.0337 | 1.1617 | 0.9725 | 0.9157 | 0.7577 |
| 2-butanone | 303 | 0.7999 | 0.9369 | 0.7415 | 0.7151 | 0.6649 |
| 2-methylpropan-2-ol(t-butyl-alcohol) | 298 | 0.7887 | 0.9207 | 0.7084 | 0.6417 | 0.5987 |
| acetic-acid | 303 | 1.0446 | 1.1786 | 1.03467 | 1.0046 | 1.0155 |
| acetone | 303 | 0.7845 | 0.9535 | 0.743 | 0.7063 | 0.6868 |
| acetonitrile | 298 | 0.7857 | 0.6687 | 0.6807 | 0.745 | 0.5307 |
| acetophenone | 298 | 1.0281 | 1.1391 | 1.0115 | 0.9654 | 0.8751 |
| benzamide | 408 | 1.0792 | 1.2292 | 1.0519 | 0.9958 | 0.9472 |
| benzene | 298 | 0.8765 | 0.9975 | 0.8225 | 0.7948 | 0.6885 |
| benzenthiol | 298 | 1.0775 | 1.2065 | 1.1055 | 1.0301 | 0.6715 |
| bromobenzene | 298 | 1.495 | | 1.5656 | 1.3959 | 1.114 |
| carbon-tetrachloride(tetrachloro-methane) | 298 | 1.594 | 1.5606 | 1.487 | 1.6578 | 1.155 |
| chlorobenzene | 298 | 1.1058 | 1.2178 | 1.0835 | 1.0471 | 0.8508 |
| chloroform(trichloro-methane) | 303 | 1.4788 | 1.8618 | 1.4604 | 1.4547 | 1.0748 |
| cyclohexane | 303 | 0.7739 | | 0.7585 | 0.6399 | 0.3729 |
| dibromo-methane | 298 | 2.4969 | | 2.8449 | 2.4344 | 1.7749 |
| dichloromethane(methylene-chloride) | 298 | 1.3266 | 1.8656 | 1.3006 | 1.2541 | 0.8806 |
| diethyl-ether | 298 | 0.7138 | 0.8828 | 0.6822 | 0.6088 | *0.1708* |
| diethylene-glycol-dimethyl-ether | 298 | 0.9434 | 1.0964 | 0.9107 | 0.8304 | 0.6804 |
| diethylene-glycol | 293 | 1.1197 | 1.2347 | 1.072 | 1.0487 | 0.9857 |
| dimethyl-sulfide | 298 | 0.8483 | 0.9121 | 0.8027 | 0.7323 | *0.0093* |
| dimethyl-sulfoxide | 303 | 1.101 | 1.1979 | 0.969 | 1.022 | 0.916 |
| ethanol | 298 | 0.7893 | 0.9053 | 0.7418 | 0.713 | 0.6323 |
| ethyl-acetate | 298 | 0.90032 | 1.05532 | 0.89022 | 0.88072 | 0.82222 |
| ethylene-glycol | 298 | 1.1135 | 1.2128 | 1.073 | 1.0561 | 1.0244 |
| fluorobenzene | 298 | 1.0225 | 1.1555 | 0.8925 | 0.942 | 0.8445 |

**Table S2: Liquid solvent densities for organic models. Italics indicate the system vaporized over the course of the simulation.**

| System | T (K) | Expt | QRNN | Organic_MPNICE | Organic_Crystals_MPNICE(wB97X) | Organic_Crystals_MPNICE(PBE) |
|---|---|---|---|---|---|---|
| formaldehyde | 258 | 0.815 | 1.161 | 0.904 | 0.9099 | 0.651 |
| glycerin | 298 | 1.2613 | 1.3286 | 1.2287 | 1.2016 | 1.1553 |
| hexamethylphosphoramide | 298 | 1.03 | 1.158 | 0.9892 | 0.825 | 0.659 |
| hexane | 298 | 0.6606 | 0.6981 | 0.6406 | 0.568 | 0.3286 |
| methanethiol | 298 | 0.8665 | 0.83 | 0.771 | 0.7707 | *0.0035* |
| methanol | 298 | 0.7914 | 0.9044 | 0.7584 | 0.6963 | 0.6544 |
| methoxybenzene(anisole) | 298 | 0.994 | 1.097 | 0.9503 | 0.8986 | 0.795 |
| methyl-acetate | 298 | 0.9342 | 1.1252 | 0.92697 | 0.9127 | 0.8715 |
| methyl-benzoate | 303 | 1.0837 | 1.1927 | 1.0457 | 1.015 | 0.9047 |
| methyl-t-butyl-ether(tert-butyl-methyl-ether) | 303 | 0.7353 | 0.8863 | 0.6754 | 0.5743 | 0.4273 |
| morpholine | 298 | 1.0005 | 1.1475 | 0.9854 | 0.8755 | 0.7235 |
| N-methyl-2-pyrolidone | 303 | 1.023 | 1.167 | 0.9667 | 0.932 | 0.84 |
| N,N-dimethylformamide | 303 | 0.9445 | 1.1125 | 0.846 | 0.8715 | 0.7845 |
| nitro-methane | 298 | 1.1371 | 1.2711 | 1.0141 | 1.1149 | 0.9741 |
| nitrobenzene | 298 | 1.2037 | 1.2307 | 1.1667 | 1.1776 | 1.0427 |
| pyridine | 298 | 0.9819 | 1.0969 | 0.9306 | 0.9232 | 0.7869 |
| quinoline | 293 | 1.0977 | 1.1945 | 1.0543 | 1.0227 | 0.9017 |
| tetrahydrofuran | 303 | 0.8833 | 1.0193 | 0.8281 | 0.7848 | 0.5843 |
| thioanisole(methyl-thio-benzene) | 298 | 1.0579 | 1.1563 | 1.039 | 0.9968 | 0.7929 |
| thiophene | 298 | 1.0649 | 1.1659 | 1.0907 | 1.0068 | 0.7899 |
| toluene | 298 | 0.8668 | 0.9728 | 0.8502 | 0.7894 | 0.6548 |
| triethylamine | 298 | 0.7275 | 0.8865 | 0.7138 | 0.6025 | 0.3685 |
| water | 298 | 0.998 | 1.163 | 0.9336 | 0.9724 | 1.159 |
| ethylene-carbonate | 317 | 1.3214 | 1.2912 | 1.2895 | 1.282 | 1.1824 |
| propylene-carbonate | 298 | 1.2047 | 1.2449 | 1.1526 | 1.1428 | 1.0757 |
| vinylene-carbonate(1,2-dioxol-2-one) | 303 | 1.35 | 1.161 | 1.2906 | 1.35555 | 1.2867 |
| dimethyl-carbonate | 303 | 1.0636 | 1.1946 | 1.0526 | 1.0333 | 0.9436 |
| ethylmethyl-carbonate | 298 | 1.012 | 1.139 | 0.9971 | 0.964 | 0.869 |
| diethyl-carbonate | 303 | 0.9692 | 1.1032 | 0.9427 | 0.916 | 0.8342 |
| FEC | 298 | 1.485 | 1.4542 | 1.4073 | 1.3982 | 1.343 |
| 1,3-dioxolane | 298 | 1.0602 | 1.1812 | 0.9724 | 0.9572 | 0.8112 |

## Table S3: Liquid solvent densities for inorganic and hybrid models

| System | T (K) | Expt | Inorganic_MPNICE | Hybrid_MPNICE_I | Hybrid_MPNICE | Hybrid_MPNICE_O |
|---|---|---|---|---|---|---|
| 1-butanol | 298 | 0.8095 | 0.5785 | | | 0.9865 |
| 1-propanol | 303 | 0.7997 | 0.5797 | | 1.0057 | 0.9787 |
| 1,2-dichloroethane | 303 | 1.2454 | 0.1154 | 1.4784 | 1.4894 | 1.4574 |
| 1,2-dimethoxy-ethane | 303 | 0.8637 | 0.7517 | | 0.0147 | 1.1067 |
| 1,2-dimethylbenzene(o-xylene) | 278 | 0.8802 | 0.7202 | 1.0792 | 1.0682 | 1.0872 |
| 1,4-dioxane | 298 | 1.0337 | 0.7027 | 1.2247 | 1.2737 | 1.2247 |
| 2-butanone | 303 | 0.7999 | 0.5859 | 1.0629 | 1.0449 | 1.0219 |
| 2-methylpropan-2-ol(t-butyl-alcohol) | 298 | 0.7887 | 0.0737 | | 0.9707 | 0.9677 |
| acetic-acid | 303 | 1.0446 | 0.7006 | 1.2976 | 1.3096 | 1.2486 |
| acetone | 303 | 0.7845 | 0.6725 | 1.0535 | 1.0235 | 1.0145 |
| acetonitrile | 298 | 0.7857 | 0.7467 | 1.0187 | 0.9927 | 0.9887 |
| acetophenone | 298 | 1.0281 | 0.8271 | 1.2131 | 1.2161 | 1.2061 |
| benzamide | 408 | 1.0792 | 0.8562 | 1.2592 | 1.2992 | 1.2612 |
| benzene | 298 | 0.8765 | 0.6915 | 1.0625 | 1.0645 | 1.0225 |
| benzenthiol | 298 | 1.0775 | 0.8875 | 1.2975 | 1.3215 | 1.2535 |
| bromobenzene | 298 | 1.495 | 1.069 | 1.787 | 1.774 | 1.728 |
| carbon-tetrachloride(tetrachloro-methane) | 298 | 1.594 | 1.027 | 0.014 | 0.792 | 1.162 |
| chlorobenzene | 298 | 1.1058 | 0.8928 | 1.3528 | 1.3398 | 1.3138 |
| chloroform(trichloro-methane) | 303 | 1.4788 | 0.0088 | 1.7748 | 0.2888 | 1.0638 |
| cyclohexane | 303 | 0.7739 | 0.0629 | | | |
| dibromo-methane | 298 | 2.4969 | 0.0369 | 0.7169 | 1.4669 | 2.0219 |
| dichloromethane(methylene-chloride) | 298 | 1.3266 | 0.0166 | 1.5646 | 0.5736 | 1.2545 |
| diethyl-ether | 298 | 0.7138 | 0.5228 | | 0.9638 | 0.9768 |
| diethylene-glycol-dimethyl-ether | 298 | 0.9434 | 0.7804 | | 1.1614 | 1.1614 |
| diethylene-glycol | 293 | 1.1197 | 0.8717 | | | 1.2337 |
| dimethyl-sulfide | 298 | 0.8483 | 0.0053 | 0.937 | 1.1183 | 0.9503 |
| dimethyl-sulfoxide | 303 | 1.101 | 0.715 | 1.292 | 1.362 | 0.981 |
| ethanol | 298 | 0.7893 | 0.6173 | 1.0243 | 0.9943 | 0.9613 |
| ethyl-acetate | 298 | 0.90032 | 0.73432 | 1.14532 | 1.17432 | 1.14132 |
| ethylene-glycol | 298 | 1.1135 | 0.8615 | | | 1.1781 |
| fluorobenzene | 298 | 1.0225 | 0.8115 | 1.2845 | 1.2605 | 1.2425 |

## Table S3: Liquid solvent densities for inorganic and hybrid models

| System | T (K) | Expt | Inorganic_MPNICE | Hybrid_MPNICE_I | Hybrid_MPNICE | Hybrid_MPNICE_O |
|---|---|---|---|---|---|---|
| formaldehyde | 258 | 0.815 | 0.703 | 1.155 | 1.152 | 1.115 |
| glycerin | 298 | 1.2613 | 1.0053 | | | 1.3204 |
| hexamethylphosphoramide | 298 | 1.03 | 0.02 | 1.195 | 1.226 | 1.0842 |
| hexane | 298 | 0.6606 | 0.0076 | 0.8556 | | 0.8806 |
| methanethiol | 298 | 0.8665 | 0.0825 | 0.8864 | 1.0495 | 0.9565 |
| methanol | 298 | 0.7914 | 0.7555 | 1.0524 | 1.0024 | 0.8369 |
| methoxybenzene(anisole) | 298 | 0.994 | 0.773 | 1.161 | 1.183 | 1.153 |
| methyl-acetate | 298 | 0.9342 | 0.8466 | 1.1542 | 1.2022 | 1.1542 |
| methyl-benzoate | 303 | 1.0837 | 0.9217 | 1.2457 | 1.2897 | 1.2647 |
| methyl-t-butyl-ether(tert-butyl-methyl-ether) | 303 | 0.7353 | 0.6382 | 1.0063 | 0.9433 | 0.9583 |
| morpholine | 298 | 1.0005 | 0.0565 | 1.1465 | 1.1555 | 1.1255 |
| N-methyl-2-pyrolidone | 303 | 1.023 | 0.693 | 1.215 | 1.21 | 1.163 |
| N,N-dimethylformamide | 303 | 0.9445 | 0.7435 | 1.1245 | 1.1135 | 1.0665 |
| nitro-methane | 298 | 1.1371 | 0.7701 | 1.3811 | 1.2092 | 1.3681 |
| nitrobenzene | 298 | 1.2037 | 0.9527 | 1.3967 | 1.4217 | 1.3607 |
| pyridine | 298 | 0.9819 | 0.6559 | 1.1619 | 1.1589 | 1.0969 |
| quinoline | 293 | 1.0977 | 0.7967 | 1.2457 | 1.2867 | 1.2137 |
| tetrahydrofuran | 303 | 0.8833 | 0.4743 | 1.0713 | 1.0963 | 1.0653 |
| thioanisole(methyl-thio-benzene) | 298 | 1.0579 | 0.8129 | 1.2359 | 1.2669 | 1.2039 |
| thiophene | 298 | 1.0649 | 0.8859 | 1.2989 | 1.3989 | 1.2409 |
| toluene | 298 | 0.8668 | 0.6978 | 1.0698 | 1.0578 | 1.0658 |
| triethylamine | 298 | 0.7275 | 0.0105 | | | |
| water | 298 | 0.998 | 0.9284 | | 1.201 | 0.858 |
| ethylene-carbonate | 317 | 1.3214 | 1.1354 | 1.4087 | 1.4324 | 1.4394 |
| propylene-carbonate | 298 | 1.2047 | 1.0557 | 1.4497 | 1.3427 | 1.3847 |
| vinylene-carbonate(1,2-dioxol-2-one) | 303 | 1.35 | 1.14 | 1.383 | 1.452 | 1.17 |
| dimethyl-carbonate | 303 | 1.0636 | 1.0756 | 1.2606 | 0.6656 | 1.2326 |
| ethylmethyl-carbonate | 298 | 1.012 | 0.9464 | 1.286 | 0.825 | 1.223 |
| diethyl-carbonate | 303 | 0.9692 | 0.8332 | 1.2622 | 1.1682 | 1.2062 |
| FEC | 298 | 1.485 | 1.237 | 1.725 | 0.993 | 1.621 |
| 1,3-dioxolane | 298 | 1.0602 | 0.7222 | 1.3332 | 1.2842 | 1.2972 |

# S7 TorsionNet500 DLPNO-CCSD(T) details

DLPNO-CCSD(T), with extrapolated cc-pVTZ/cc-pVQZ CBS energy, is run with the ORCA software package,[5] version 6.0.1. All the TorsionNet500 structures are netural, closed-shell and use RHF as the reference. The CBS extrapolation exponents are the defaults[6] for the ORCA package.

An example input file can be found below:

```
!DLPNO-CCSD(T) Extrapolate(3/4,cc) cc-pVQZ/C TightSCF PAL4


%MaxCore 10000


%scf
maxiter 500
end


*xyzfile 0 1 FILENAME.xyz
```

# S8 Water hydration free energy details

The hydration free energy calculation was performed using the free energy perturbation (FEP) method. Following Beutler *et al.*,[7] we utilize a soft-core Lennard-Jones (LJ) potential,

$$V_{scLJ}(r,\lambda;\alpha,p) = 4\epsilon(1-\lambda)\left(\frac{1}{\left[\alpha\lambda^p + \left(\frac{r}{\sigma}\right)^6\right]^2} - \frac{1}{\alpha\lambda^p + \left(\frac{r}{\sigma}\right)^6}\right), \tag{S1}$$

where $p = 1$ and $\alpha = 0.5$ are used in this work. The thermodynamic cycle connecting the initial state (vacuum) and the final state (solution) consists of two key steps. In the first step the soft-core LJ potential is turned on between the solute and solvent using the OPLS_2005[8] LJ parameters ($\epsilon$ and $\sigma$),

$$E(\lambda_1) = E_{solute} + E_{solvent} + V_{scLJ}(\lambda_1). \tag{S2}$$

In the second step, the soft-core LJ interaction is replaced with the true solute-solvent interaction, as described by the

Organic_MPNICE model,

$$E(\lambda_2) = (1-\lambda_2)E_{solute} + (1-\lambda_2)E_{solvent} + \lambda_2 E_{complex} + V_{scLJ}(\lambda_2). \tag{S3}$$

Note that in this definition $V_{scLJ}(\lambda = 1) = 0$ and $V_{scLJ}(\lambda = 0)$ represents the full LJ potential.

The initial cubic water box structure was generated using System Builder in the Schrödinger suite, with a side length of 19.0 Å. The simulations were performed using the OpenMM software.[9] The following $\lambda$ schedule was employed: $\lambda_1 = 1.0, 0.92, 0.84, 0.76, 0.68, 0.6, 0.45, 0.3, 0.15, 0.0$ for step 1 and $\lambda_2 = 0.0, 0.14285714, 0.28571429, 0.42857143, 0.57142857, 0.71428571, 0.85714286, 1.0$ for step 2. At each $\lambda$ value, a 250 ps Langevin dynamics simulation with a Monte Carlo barostat was conducted at 298.15 K and 1 atmosphere, using a time step of 0.5 fs, following a 10 ps pre-equilibration run. During the 250 ps production run, Hamiltonian replica exchange between neighboring replicas was attempted every 1000 steps (0.5 ps). The final free energy was computed using MBAR,[10] based on the last 200 ps of the simulation. A full report on this method and it's application to hydration free energies of organic molecules is forthcoming.

# S9 NaCl electric response

Fixed ion dielectric tensor and Born Effective Charges for NaCl using Inorganic_MPNICE. Off diagonal terms in $\epsilon^{\infty}_{\alpha\beta}$ are caused by restricting Qeq to atomic point charges.

$$\epsilon^{\infty}_{\alpha\beta} = \begin{pmatrix} 1.67 & 0.39 & -0.55 \\ 0.39 & 1.23 & -0.32 \\ -0.55 & -0.32 & 1.45 \end{pmatrix} \tag{S4}$$

$$Z^{*}_{i\alpha\beta}(\mathrm{Na}) = -Z^{*}_{i\alpha\beta}(\mathrm{Cl}) = \begin{pmatrix} 0.774 & 0.0 & 0.0 \\ 0.0 & 0.774 & 0.0 \\ 0.0 & 0.0 & 0.774 \end{pmatrix} \tag{S5}$$

# S10 Phonon Calculations

The MDR benchmark was run with an optimization threshold of 0.01 eV/A, using the FIRE algorithm with the FrechetCellFilter in ASE. Thermal properties were obtained using phonopy[11,12] after optimization. The non-analytic correction for NaCl was additionally computed via the phonopy implementation, using computed dielectric and Born effective charges for the single unit cell as input.

# S11 LiAlO2 data

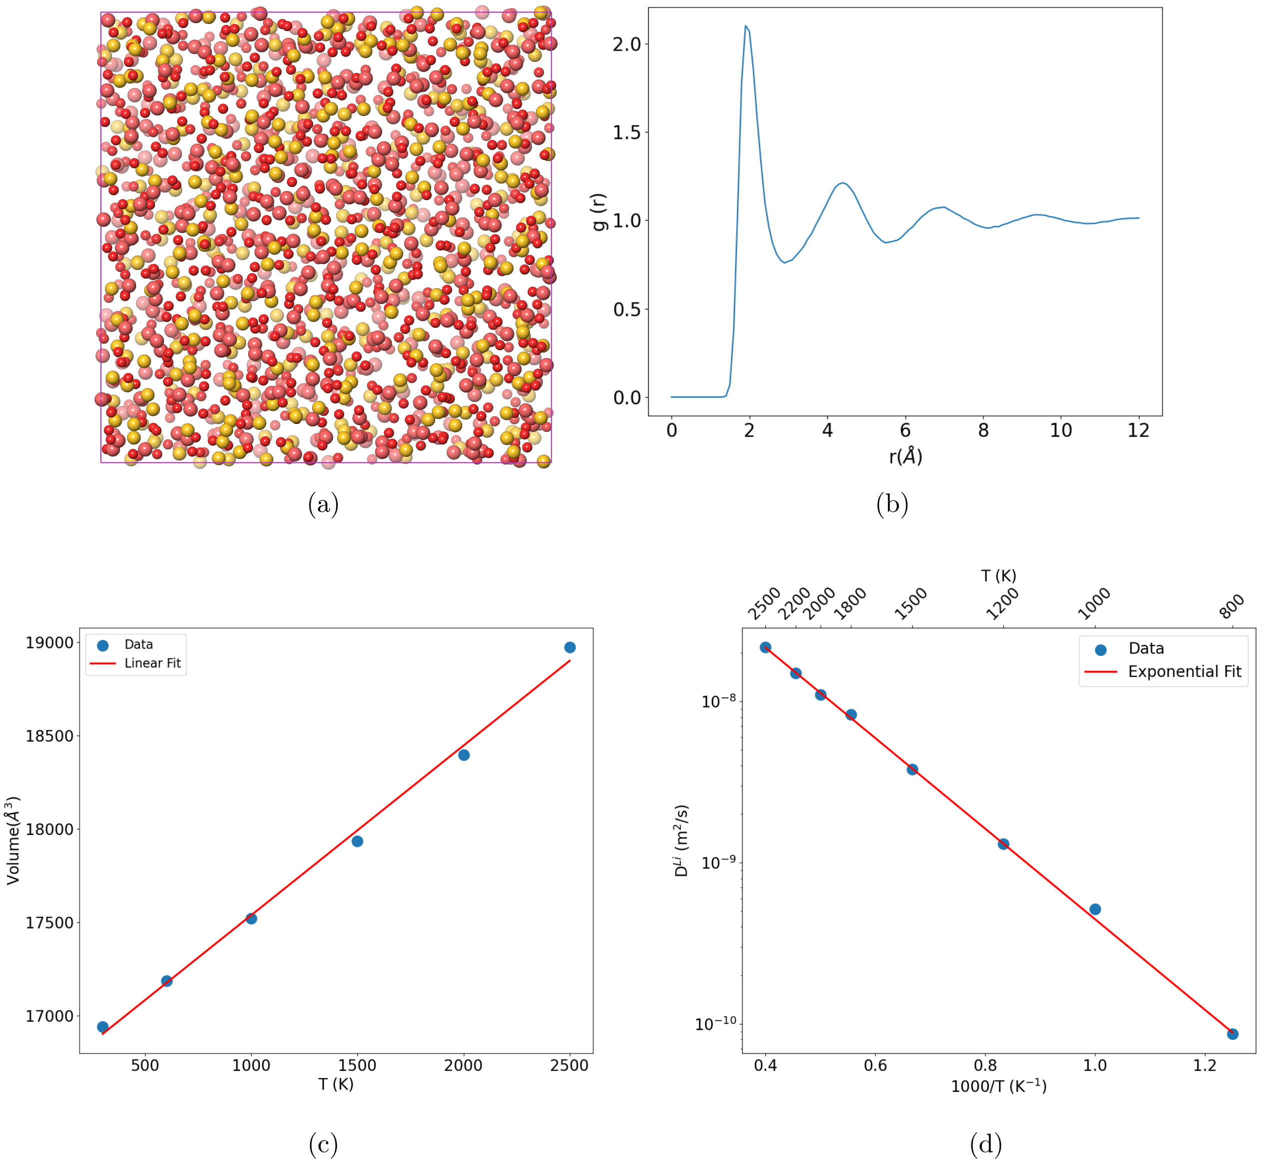


Figure S2: (a) Snapshot of the amorphous phase of LiAlO2 obtained after 500 ps equilibration at 2800 K. (b) Li-O radial distribution function (rdf) plot of the amorphous structure of LiAlO2 at 2800 K. (c) Average volume of the supercell as a function of temperature for crystal phase of LiAlO2. (d) Li ion diffusivity as a function of inverse of the temperature (1000/T) in the amorphous phase of LiAlO2.

# References


(1) Irwin, J. J.; Tang, K. G.; Young, J.; Dandarchuluun, C.; Wong, B. R.; Khurelbaatar, M.; Moroz, Y. S.; Mayfield, J.; Sayle, R. A. ZINC20—a free ultralarge-scale chemical database for ligand discovery. *Journal of chemical information and modeling* **2020**, *60*, 6065–6073.

(2) Jacobson, L. D.; Stevenson, J. M.; Ramezanghorbani, F.; Ghoreishi, D.; Leswing, K.; Harder, E. D.; Abel, R. Transferable neural network potential energy surfaces for closed-shell organic molecules: Extension to ions. *Journal of Chemical Theory and Computation* **2022**, *18*, 2354–2366.

(3) Wahl, O.; Sander, T. Tautobase: An open tautomer database. *Journal of Chemical Information and Modeling* **2020**, *60*, 1085–1089.

(4) Zhou, D.; Bier, I.; Santra, B.; Jacobson, L. D.; Wu, C.; Garaizar Suarez, A.; Almaguer, B. R.; Yu, H.; Abel, R.; Friesner, R. A. et al. A robust crystal structure prediction method to support small molecule drug development with large scale validation and blind study. *Nat. Commun.* **2025**, *16*.

(5) Neese, F. The ORCA program system. *Wiley Interdiscip. Rev.: Comput. Mol. Sci.* **2012**, *2*, 73–78.

(6) Neese, F.; Valeev, E. F. Revisiting the Atomic Natural Orbital Approach for Basis Sets: Robust Systematic Basis Sets for Explicitly Correlated and Conventional Correlated ab initio Methods? *J. Chem. Theory Comput.* **2011**, *7*, 33–43.

(7) Beutler, T. C.; Mark, A. E.; van Schaik, R. C.; Gerber, P. R.; Van Gunsteren, W. F. Avoiding singularities and numerical instabilities in free energy calculations based on molecular simulations. *Chemical physics letters* **1994**, *222*, 529–539.

(8) Banks, J. L.; Beard, H. S.; Cao, Y.; Cho, A. E.; Damm, W.; Farid, R.; Felts, A. K.; Halgren, T. A.; Mainz, D. T.; Maple, J. R. et al. Integrated modeling program, applied chemical theory (IMPACT). *Journal of computational chemistry* **2005**, *26*, 1752–1780.

(9) Eastman, P.; Galvelis, R.; Peláez, R. P.; Abreu, C. R.; Farr, S. E.; Gallicchio, E.; Gorenko, A.; Henry, M. M.; Hu, F.; Huang, J. et al. OpenMM 8: molecular dynamics simulation with machine learning potentials. *The Journal of Physical Chemistry B* **2023**, *128*, 109–116.

(10) Shirts, M. R.; Chodera, J. D. Statistically optimal analysis of samples from multiple equilibrium states. *The Journal of chemical physics* **2008**, *129*.

(11) Togo, A.; Chaput, L.; Tadano, T.; Tanaka, I. Implementation strategies in phonopy and phono3py. *J. Phys. Condens. Matter* **2023**, *35*, 353001.

(12) Togo, A. First-principles Phonon Calculations with Phonopy and Phono3py. *J. Phys. Soc. Jpn.* **2023**, *92*, 012001.
